# Supplementary material for: Improving Conversational Recommendation Systems' Quality with Context-Aware Item Meta Information
Source: arXiv:2112.08140 source file (2021-12-15)
Supplement: Supplementary file 1 [file appendix.tex]

\textbf{The trade-off between language generation and recommendation during traning.} We separate language training objective from the jointly trained loss and compare the trained models on language generation metrics on ReDial in table \ref{tab:language_ablation}. \textbf{ALISE-L} denotes the model trained with only the language generation objective $Loss_l$ from equation (\ref{loss:language}). 

\begin{table}[!ht]
	\centering
	\caption{Results of \textbf{ALISE} and \textbf{ALISE-L} on ReDial.}
	\begin{tabularx}{1.0\columnwidth}{cccccc}
		\hline
		Model & Dist2 & Dist4 & Bleu2 & Bleu4 \\
		\hline
		ALISE-L     & \bf{1.13} & \bf{2.12} & \bf{0.295} & \bf{0.171} \\
		ALISE       & 0.822 & 1.313 & 0.246 & 0.143 \\
        \hline
    \end{tabularx}
    \label{tab:language_ablation}
\end{table}

As we can see, training only on language generation objective yields better results. In the settings of \textbf{ALISE}, both tasks update the weights of the same pre-trained language model simultaneously with different goals: In recommendation, the language model needs to construct meaningful scores for generated candidates; In response generation, the language model aims to generate next token given previous contexts. This experiment showed that this joint training approach induces a trade-off between training on response generation and recommendation: back-propagation on the recommendation objective can lead to catastrophic forgetting of information learned from pre-training, which leads to worse language metrics.
